# Supplementary material for: Why Don't You Clean Your Glasses? Perception Attacks with Dynamic Optical Perturbations
Source: arXiv:2307.13131 source file (2023-07-27)
Supplement: Supplementary file 1 [file appendix.tex]

\appendix
\label{sec:appendix}
\section{Ablation Study on \name}
We perform an ablation study to investigate the contributions of \namenospace's components toward the final attack performance. We first consider the effect of removing TNet in \namenospace/d, i.e., when optimizing for an adversarial perturbation, we use $I_d$ directly as $I_p$ without passing it through TNet. We also consider the effectiveness of randomly generated perturbations in \namenospace/r. For \namenospace/r, we randomly generate 20 perturbations to attack the signs and select the perturbation with the highest ASR. Finally, we study the contribution from considering the variation of environmental factors. For this study, we fix all the factors, e.g., background, perspective, rotation, distance, and the light conditions, when preparing data to optimize a perturbation model using \namenospace/s. We report the results in Figure~\ref{fig:ablation}. For all three models, the comprehensive \name achieves significantly better results. Random perturbations perform the worst among all the variants except for ResNet-50. This can again be explained by the fact that classifiers are in general easier to attack when compared to object detectors~\cite{chen2018shapeshifter}. Some random guesses might fall inside vulnerable regions of the model's loss surface. However, the attack performance is still far from the performance of our approach. For \namenospace/s, not considering the environmental factors when crafting the perturbation results in highly sensitive perturbations with unstable attack performance. This is more obvious when the ambient light is stronger -- above $1500$ lux the perturbations have no effect.

\begin{figure*}[h]
\resizebox{!}{.28\linewidth}{%
\begin{tikzpicture}
\begin{axis}[
    xlabel={Illuminance (lux)},
    ylabel={Attack Success Rate (\%)},
    xmin=0, xmax=3000,
    ymin=0, ymax=100,
    xtick={0, 500, 1000, 1500, 2000, 2500, 3000},
    ytick={0, 20, 40, 60, 80, 100},
    legend pos=south east,
    legend style={at={(axis cs:2800,50)},anchor=north east},
    ymajorgrids=true,
    grid style=dashed,
    % scale=0.66
    title=ResNet-50,
]
    \addplot [color=blue, mark=square] table [x=illuminance, y=asr, col sep=comma] {Data/cat_resnet50.csv};
    
    \addplot [color=green, mark=*] table [x=illuminance, y=asr, col sep=comma] {Data/abl_resnet50_d.csv};

    \addplot [color=brown, mark=+] table [x=illuminance, y=asr, col sep=comma] {Data/abl_resnet50_r.csv};
    
    \addplot [color=red, mark=o] table [x=illuminance, y=asr, col sep=comma] {Data/abl_resnet50_s.csv};
    
    \legend{\namenospace, \namenospace/d, \namenospace/r, \namenospace/s}

\end{axis}
\end{tikzpicture}
}
\resizebox{!}{.28\linewidth}{%
\begin{tikzpicture}
\begin{axis}[
    xlabel={Illuminance (lux)},
    xmin=0, xmax=3000,
    ymin=0, ymax=100,
    xtick={0, 500, 1000, 1500, 2000, 2500, 3000},
    ytick={0, 20, 40, 60, 80, 100},
    legend pos=north east,
    legend style={at={(axis cs:2800,75)},anchor=north east},
    ymajorgrids=true,
    grid style=dashed,
    % scale=0.66
    title=Faster R-CNN,
]
    \addplot [color=blue, mark=square] table [x=illuminance, y=asr, col sep=comma] {Data/cat_fasterrcnn.csv};
    
    \addplot [color=green, mark=*] table [x=illuminance, y=asr, col sep=comma] {Data/abl_fasterrcnn_d.csv};

    \addplot [color=brown, mark=+] table [x=illuminance, y=asr, col sep=comma] {Data/abl_fasterrcnn_r.csv};
    
    \addplot [color=red, mark=o] table [x=illuminance, y=asr, col sep=comma] {Data/abl_fasterrcnn_s.csv};
    
    \legend{\namenospace, \namenospace/d, \namenospace/r, \namenospace/s}
\end{axis}
\end{tikzpicture}
}
\resizebox{!}{.28\linewidth}{%
\begin{tikzpicture}
\begin{axis}[
    xlabel={Illuminance},
    xmin=0, xmax=3000,
    ymin=0, ymax=100,
    xtick={0, 500, 1000, 1500, 2000, 2500, 3000},
    ytick={0, 20, 40, 60, 80, 100},
    legend pos=north east,
    legend style={at={(axis cs:2800,75)},anchor=north east},
    ymajorgrids=true,
    grid style=dashed,
    title=YOLO v3,
    %height=2in,
    %width=3.5in,
    % scale=0.66
]
    \addplot [color=blue, mark=square] table [x=illuminance, y=asr, col sep=comma] {Data/cat_yolo.csv};
        
    \addplot [color=green, mark=*] table [x=illuminance, y=asr, col sep=comma] {Data/abl_yolo_d.csv};

    \addplot [color=brown, mark=+] table [x=illuminance, y=asr, col sep=comma] {Data/abl_yolo_r.csv};
    
    \addplot [color=red, mark=o] table [x=illuminance, y=asr, col sep=comma] {Data/abl_yolo_s.csv};
    
    \legend{\namenospace, \namenospace/d, \namenospace/r, \namenospace/s}
    
\end{axis}
\end{tikzpicture}
}
\caption{Ablation study results to observe the contribution of different components of \namenospace. \namenospace/r represents randomly generated perturbations, \namenospace/d represents a perturbation without TNet, and \namenospace/s represents a perturbation trained with fixed environmental factors (e.g., background, distance, perspective, rotation, distance, and light condition).}
\label{fig:ablation}
\end{figure*}

\section{Evaluation Against Defense: Feature Squeezing}
In this section, we study the effectiveness of a defense solution feature squeezing against our attack. We evaluate the effectiveness of bit-depth reduction on our adversarial perturbations by comparing its impact on classifier accuracy for benign and adversarial samples. The results are shown in Figure~\ref{fig:feature-sq}.

As the input image bit depth decreases, both benign and adversarial classifier accuracy remains relatively stable until the bit depth drops below 2 bits/channel. At this point, we observe a general increase in adversarial accuracy.
We hypothesize that this is due to the dot perturbation's color robustness -- each dot maintains a constant color gradually fading outwards. As a result, decreasing the bit-depth only slightly attenuates the perturbation until the final step, in which each channel only has 2 possible values, more significantly affecting the perturbation.

\begin{figure}[h]
\begin{tikzpicture}
\begin{axis}[
    title={Bit-Depth Feature Squeezing (Stop Sign)},
    xlabel={Image Depth (bits/channel)},
    ylabel={Classifier Accuracy (\%)},
    xmin=.5, xmax=8.5,
    ymin=-5, ymax=105,
    xtick={8,7,6,5,4,3,2,1},
    ytick={0, 10,20,30,40,50,60,70,80,90,100},
    %legend pos= north east,
    %legend style={at={(axis cs:8,50)},anchor=north east},
    % legend style={nodes={scale=0.7, transform shape}},
    legend style={at={(axis cs:8,95)},anchor=north east,nodes={scale=0.7, transform shape}},
    ymajorgrids=true,
    grid style=dashed,
    height=2in,
    width=3in,
    ]
% Legend Entries
\addplot[color=blue,]
    coordinates {(-1,-1)};
\addlegendentry{benign}
\addplot[color=red,]
    coordinates {(-1,-1)};
\addlegendentry{adversarial}

%120
\addplot[color=blue, mark=pentagon,forget plot]
    coordinates {(8,100.00)(7,100.00)(6,100.00)(5,100.00)(4,100.00)(3,100.00)(2,100.00)(1,100.00)};
\addplot[color=red, mark=pentagon,]
    coordinates {(8,0.00)(7,0.00)(6,0.00)(5,0.00)(4,0.00)(3,0.00)(2,0.00)(1,5.88)};
\addlegendentry{120 lux}
    
%180
\addplot[color=blue, mark=square,forget plot]
    coordinates {(8,100.00)(7,100.00)(6,100.00)(5,100.00)(4,100.00)(3,100.00)(2,100.00)(1,100.00)};
\addplot[color=red, mark=square,]
    coordinates {(8,0.00)(7,0.00)(6,0.00)(5,0.00)(4,0.00)(3,0.00)(2,0.00)(1,40.74)};
\addlegendentry{180 lux}
    
%300
\addplot[color=blue, mark=star,forget plot]
    coordinates {(8,100.00)(7,100.00)(6,100.00)(5,100.00)(4,100.00)(3,100.00)(2,100.00)(1,100.00)};
\addplot[color=red, mark=star,]
    coordinates {(8,0.00)(7,0.00)(6,0.00)(5,0.00)(4,0.00)(3,0.00)(2,0.00)(1,15.87)};
\addlegendentry{300 lux}

%600
\addplot[color=blue, mark=triangle,forget plot]
    coordinates {(8,100.00)(7,100.00)(6,100.00)(5,100.00)(4,100.00)(3,100.00)(2,100.00)(1,100.00)};
\addplot[color=red, mark=triangle,]
    coordinates {(8,0.00)(7,0.00)(6,0.00)(5,0.00)(4,0.00)(3,0.00)(2,0.00)(1,10.14)};
\addlegendentry{600 lux}

%1500
\addplot[color=blue, mark=o,forget plot]
    coordinates {(8,100.00)(7,100.00)(6,100.00)(5,100.00)(4,100.00)(3,100.00)(2,100.00)(1,100.00)};
\addplot[color=red, mark=o,]
    coordinates {(8,7.25)(7,7.25)(6,7.25)(5,7.25)(4,7.25)(3,5.80)(2,5.80)(1,71.74)};
\addlegendentry{1500 lux}

%3000
\addplot[color=blue, mark=diamond,forget plot]
    coordinates {(8,100.00)(7,100.00)(6,100.00)(5,100.00)(4,100.00)(3,100.00)(2,100.00)(1,100.00)};
\addplot[color=red, mark=diamond,]
    %coordinates {(8,21.69)(7,21.69)(6,21.69)(5,21.69)(4,20.48)(3,20.48)(2,22.89)(1,100.00)};
    coordinates {(8,10.33)(7,10.33)(6,10.33)(5,10.80)(4,7.98)(3,6.57)(2,5.63)(1,13.15)};
\addlegendentry{3000 lux}

%\legend{Benign, Adversarial}
    
\end{axis}
\end{tikzpicture}
\caption{A comparison of classifier accuracy for benign and adversarial samples when varying image bit-depth of the RGB channels, ranging from native 8-bit color resolution (256 possible values) to 1-bit (2 possible values). Blue plots represent benign accuracy, while red plots represent adversarial examples. Different markers indicate different lux levels. 
%As bit-depth decreases, so does benign classifier accuracy. However, the classifier consistently performs poorly on adversarially perturbed inputs.
%\eric{can we include a red/blue key in the figure?}
}
\vspace{-0.1in}
\label{fig:feature-sq}
\end{figure}

\section{Measured Illuminance}
Measured illuminance of various ambient environments can be found in Tabel~\ref{tab:light}. \name can support much stronger ambient light compared to prior works.

\begin{table}[h]
\centering
\caption{The measured illuminance of various ambient environments~\cite{eun2016bright} as well as how \name and prior work were performed under each ambient light level. \Tdot~ indicates high ASR, \LEFTcircle~ indicates low to medium ASR, and \Twdot~ indicates not working at all. \name supports much stronger ambient light.}
\begin{tabular}{r|ccc}
\toprule
% \tabularnewline
Ambient Environment              & \multicolumn{1}{l}{Illuminance} & \name & SLAP \\ \hline
Indoor w/ Ceiling Lights       & 50 lux                          &    \Tdot      &   \Tdot   \\
Before Sunset & 120 lux                         &   \Tdot       &     \Tdot \\
Overcast Afternoon                      & 400-600 lux                                &    \Tdot      &   \LEFTcircle   \\
Midday, Overcast          & 1k-2k lux                   &    \Tdot      &   \Twdot   \\
Midday, Clear              &           40k-100k lux                      &    \LEFTcircle      &  \Twdot    \\ 
\bottomrule
\end{tabular}
\label{tab:light}
\end{table}
